# Supplementary material for: Physics-informed machine learning: A mathematical framework with applications to time series forecasting
Source: arXiv:2507.08906 source file (2025-07-11)
Supplement: Supplementary file 1 [file resume-fr.tex]

% !TEX root = ../main.tex
%
\chapter{Résumé}
\label{appendix:resume-fr}

The doctoral schools of Sorbonne Université require at least one page of 
summary in French.
(Even if the website says that you need to provide more than one page,
one is enough,
which I did).

Résumons donc en français. 
Tout bon résumé commence par une description générale du problème de 
la thèse.
Le problème étant que les écoles doctorales de Sorbonne Université exigent 
au moins une page de résumé en français.
Voici donc un résumé garanti non traduit sur un DeepL.

Le deuxième paragraphe du résumé doit répondre à la question 
\textit{pourquoi le(s) problème(s) présenté(s) est un vrai problème ?}.

Ensuite, le troisième paragraphe doit répondre à la question
\textit{quelles sont les solutions apportées par la thèse à ces problèmes ?}
Cette thèse explore ces problèmes en profondeur,
en étudiant l'état de l'art lié ...
et présente la solution \textit{SystèmeCool2Ouf},
conçu pour répondre aux problématiques exposées.
L'une des principales exigences est une approche \textit{DurACuir}
qui \textit{EstVraimentVraimentDureCar...}
Cependant, cela rend difficile la satisfaction des attentes en matière
de \textit{Toute solution à des petits défauts et compromis, on va pas se le 
cacher}.

Paragraphe 4, \textit{En quoi la solution est meilleure que l'état de l'art ?}
Pour répondre à ces défis,
nous avons fait le choix d'adopter une approche \textit{...}
en fournissant les plus fortes garanties de \textit{...}.
Un défi connexe est \textit{...},
que nous avons limité grâce à \textit{...}

Enfin, traditionnelement on liste une référence aux contribution,
Les contributions de cette thèse peuvent être résumées comme suit:
\begin{itemize}
    \item ...;
    \item ...;
    \item ...;
\end{itemize}

Notre évaluation expérimentale montre que ...
